# Supplementary material for: Formation of C$_{18}$H and C$_{18}$H$_2$ molecules by low energy irradiation with atomic and molecular hydrogen
Source: arXiv:2004.03291 source file (2020-04-07)
Supplement: Supplementary file 1 [file supp_mat.tex]

We provide the raw data of the potential energy curves obtained by different 
SK parameters for the considered adsorbate cites, that are graphically reported
in Sec 3.1. 
We also include the visualization of the formation of a C$_{18}$H molecule at 
2 eV by using the 3OB SK parameters with DFTD3 dispersion correction, as well as
the four different event observed during the hydrogen irradiation of the C$_{18}$ 
molecule by H$_2$ molecules.
